# Supplementary material for: Enhancing Constraint Programming via Supervised Learning for Job Shop Scheduling
Source: arXiv:2211.14492 source file (2023-04-12)
Supplement: Supplementary file 1 [file Appendix.tex]

\section*{Appendix}

\begin{figure*}[!t]
    \centering
    \resizebox{\textwidth}{!}{
    \subfloat[Cmax]{
    \includegraphics[width=0.33\textwidth]{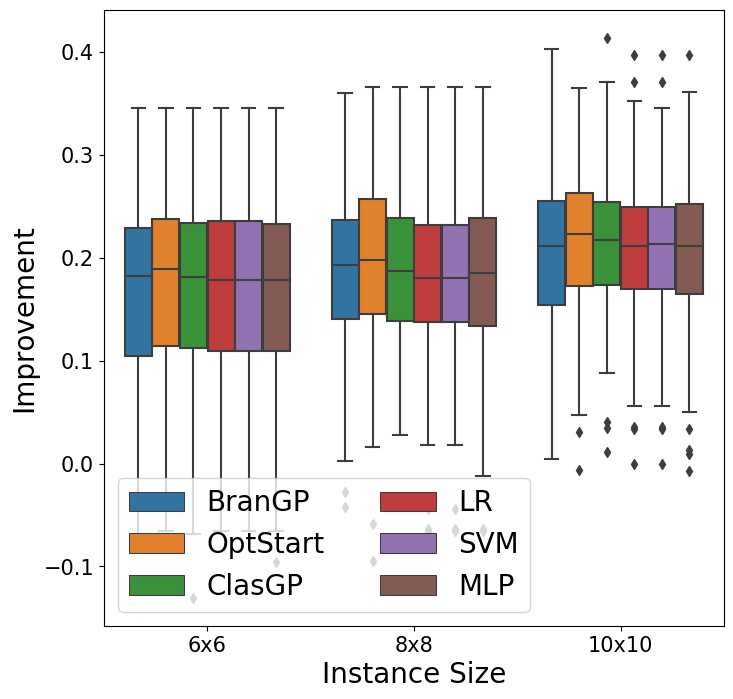}
    }
    \subfloat[Tmax]{
    \includegraphics[width=0.33\textwidth]{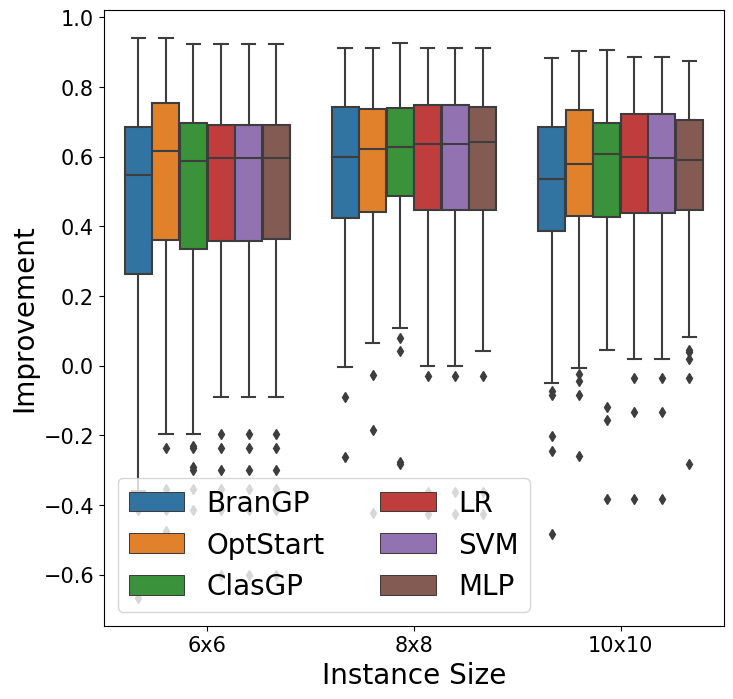}
    }
    \subfloat[TWT]{
    \includegraphics[width=0.33\textwidth]{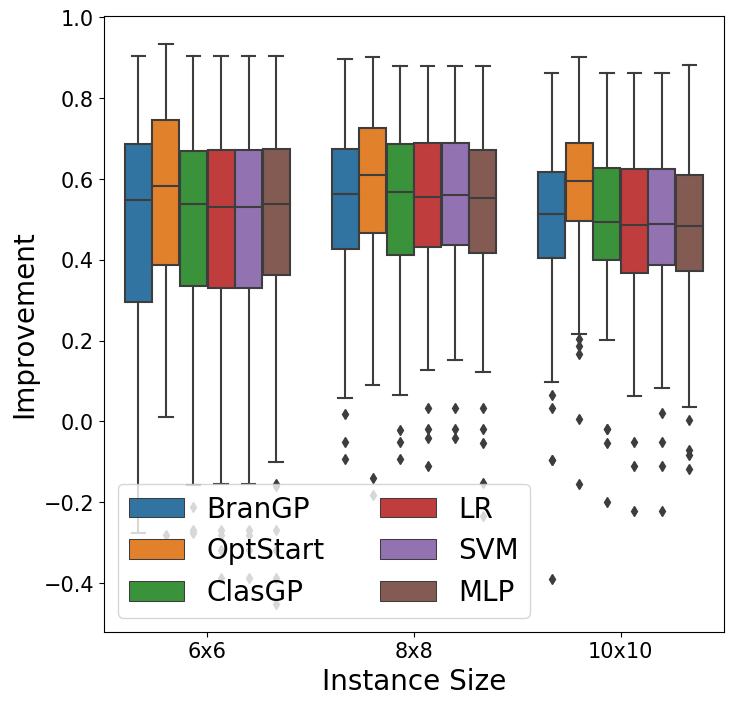}
    }
    }
    \caption{The improvement of the learning-based variable ordering methods over the default, in terms of the objective value of the initial feasible solution generated.}
    \label{fig:imp_small_ini}
\end{figure*}

\begin{figure*}[!t]
    \centering
    \resizebox{\textwidth}{!}{
    \subfloat[Cmax]{
    \includegraphics[width=0.33\textwidth]{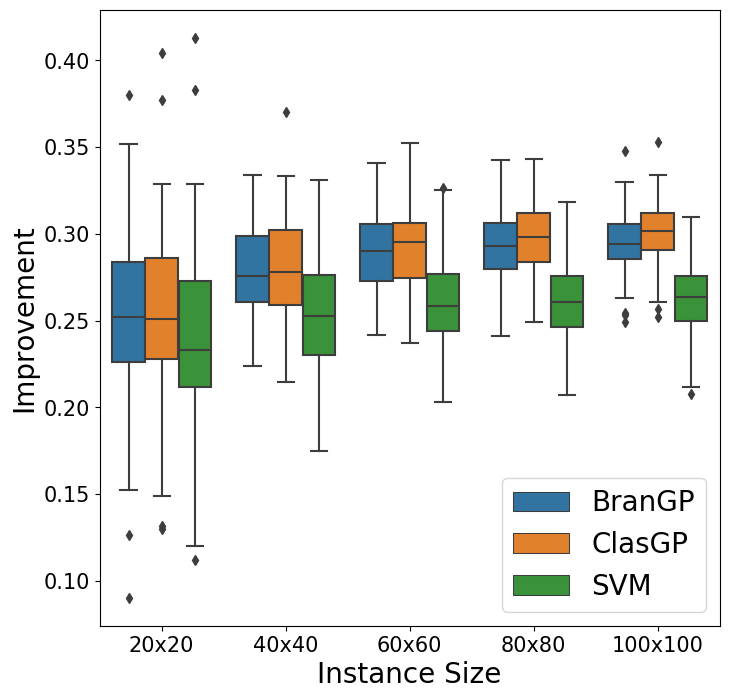}
    }
    \subfloat[Tmax]{
    \includegraphics[width=0.33\textwidth]{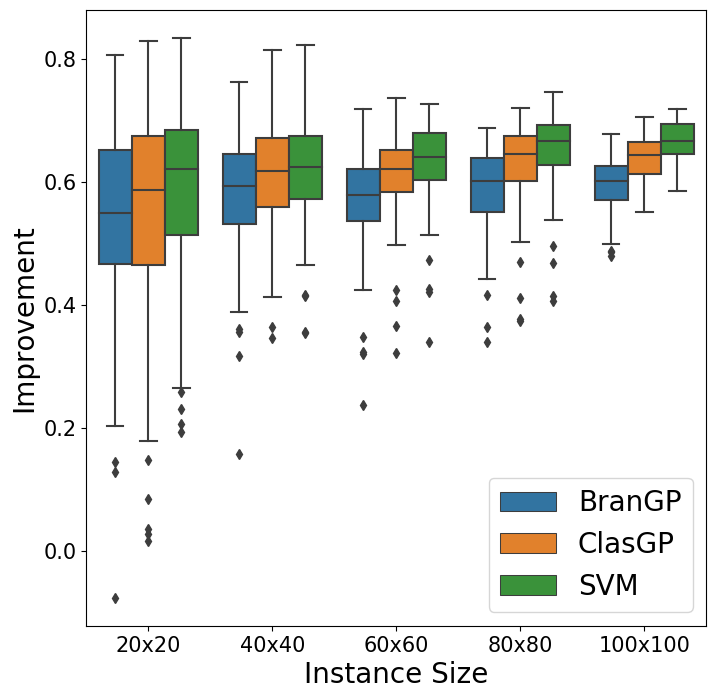}
    }
    \subfloat[TWT]{
    \includegraphics[width=0.33\textwidth]{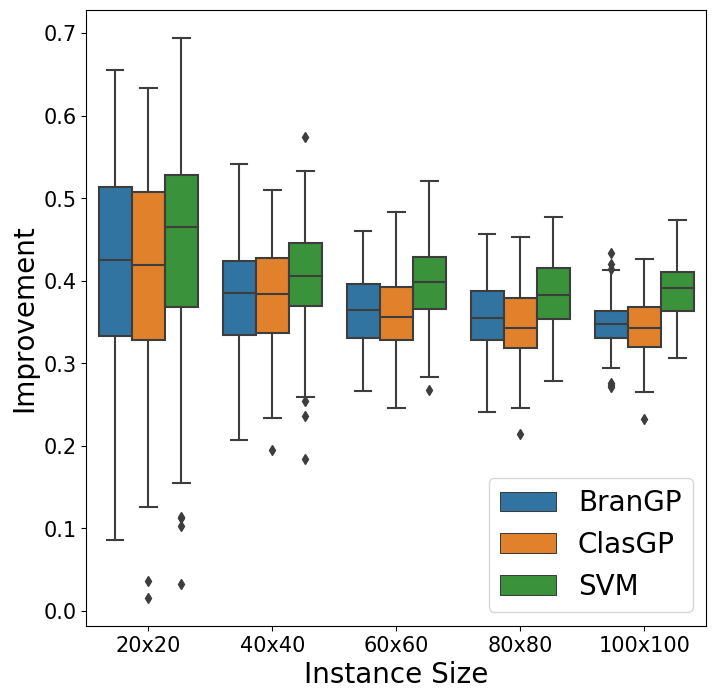}
    }
    }
    \caption{The improvement of selected learning-based variable ordering methods over the default, in terms of the objective value of the initial feasible solution generated.}
    \label{fig:large_ini}
\end{figure*}
